# Supplementary material for: Evaluating Reinforcement Learning Safety and Trustworthiness in Cyber-Physical Systems
Source: arXiv:2503.09388 source file (2025-03-12)
Supplement: Supplementary file 1 [file 7_appendix.tex]

\begin{table*}[h]
\caption{Goal 1 Responses for Case Study by C1}

\label{tab:goal1-res}
\centering
\footnotesize{ % Experimenting with small font
\begin{tabular}{p{5.5cm}|p{5.5cm}|p{5.5cm}}
\rowcolor{BlueGray} \multicolumn{3}{c}{\textbf{Goal 1: Real-World Readiness \& Adaptability}} \\
\multicolumn{3}{c}{\textbf{\texttt{Subgoal 1.1 Scenario Diversity \& Coverage}}} \\ \midrule

\textbf{\texttt{\uline{ASK 1:}} Have diverse scenarios, including standard operations, irregularities like sensor errors, and edge cases (such as abrupt environmental shifts), been comprehensively identified?} & \textbf{\texttt{\uline{ASK 2:}} Have potential adversarial scenarios been considered, including perturbations to observations, actions, or rewards?} & \textbf{\texttt{\uline{ASK 3:}} In multi-agent settings, have failures or suboptimal behaviors of other agents been considered to ensure individual RL-agents are able to adapt appropriately?} \\ 

\ding{51} \texttt{Yes} \ding{111} \texttt{No} \ding{111} \texttt{N/A} \ding{111} \texttt{?} & \ding{51} \texttt{Yes} \ding{111} \texttt{No} \ding{111} \texttt{N/A} \ding{111} \texttt{?} & \ding{51} \texttt{Yes} \ding{111} \texttt{No} \ding{111} \texttt{N/A} \ding{111} \texttt{?} \\ 

{\small \textbf{Explanation:}} \raggedright \newline  -- \textit{Normal Operations}: Standard path following with dynamic obstacle avoidance \newline  -- \textit{Abnormal Scenarios}: Sudden obstacles, sensor failures, communication delays \newline  -- \textit{Edge Cases}: High-density environments, multiple agent failures, extreme conditions & {\small \textbf{Explanation:}} \newline -- \textit{Anomaly Detection:} Continuous monitoring of state variables (e.g., agent velocities, distances to obstacles) and triggering alerts when thresholds are exceeded. & {\small \textbf{Explanation:}} \newline -- \textit{Detecting Failure:} Heartbeat signals indicate potential failure if absent. \newline -- \textit{Adapt to Failure:} Train agents for resilience and adaptability in unpredictable scenarios. \\ \hline

\multicolumn{3}{c}{\textbf{\texttt{Subgoal 1.2 Design-Environment Alignment}}} \\ \midrule

\multicolumn{3}{p{16.5cm}}{\centering \textbf{\texttt{\uline{ASK 0:}} Does the proposed RL agent align with the environment’s characteristics, such as observability, \newline continuity, and state representation?}} \\ 

\multicolumn{3}{p{16.5cm}}{\centering \ding{51} \texttt{Yes} \ding{111} \texttt{No} \ding{111} \texttt{N/A} \ding{111} \texttt{?}} \\ 

\multicolumn{3}{p{16.5cm}}{{\small \textbf{Explanation:}} \newline -- \textit{Observability:} (a) Partially Observable Markov Decision Processes (POMDPs)  (b) Implement LSTM (for noisy state inputs) \newline -- \textit{Continuous States and Actions:} (a) DDPG} \\ \hline

\multicolumn{3}{c}{\textbf{\texttt{Subgoal 1.3 Resilience \& Adaptation in Real-World Deployment}}} \\ \midrule

\textbf{\texttt{\uline{ASK 5:}} Does the RL system include mechanisms, such as anomaly detection or uncertainty estimation, to detect when the agent encounters out-of-domain states or adversarial scenarios?} & \textbf{\texttt{\uline{ASK 6:}} Is there a pre-defined strategy for handling unexpected scenarios, such as switching to a defined safe mode, halting or deferring to a human overseer?} & \textbf{\texttt{\uline{ASK 7:}} Have the accuracy and reliability of transferring policies from sim-to-real world settings been validated across all critical aspects, including sensor fidelity, environmental dynamics, and latency?} \\ 

\ding{51} \texttt{Yes} \ding{111} \texttt{No} \ding{111} \texttt{N/A} \ding{111} \texttt{?} & \ding{51} \texttt{Yes} \ding{111} \texttt{No} \ding{111} \texttt{N/A} \ding{111} \texttt{?} & \ding{51} \texttt{Yes} \ding{111} \texttt{No} \ding{111} \texttt{N/A} \ding{111} \texttt{?} \\ 

{\small \textbf{Explanation:}} \newline -- \textit{Detection of Adversarial Scenarios:} \newline Mahalanobix Distance-Based OOD Detection: Calculate the Mahalanobis distance of incoming observations from the training distribution to identify OOD scenarios. \newline -- \textit{Anomaly Detection:} Continuous monitoring of state variables (e.g., agent velocities, distances to obstacles) and trigger alerts when values exceed predefined thresholds. & {\small \textbf{Explanation:}} \newline -- \textit{Emergency Stop Mechanism:} \newline $\bullet$ Hard Constraints: Trigger an emergency stop or safe mode when critical safety thresholds (e.g., minimum separation distances) are violated. \newline $\bullet$ Abort Hover followed by Land/Human Control Fail Modes. \newline -- \textit{Fallback Policies:} \newline $\bullet$ A* with real-time obstacle avoidance \newline $\bullet$ Velocity Obstacles & {\small \textbf{Explanation:}} \newline -- \textit{Multi-Tier Training:} \newline 1. Start in low fidelity training (Pygame) \newline 2. Fine-tune on High Fidelity Simulation (Gazebo) \newline 3. Online Training (Real World). Record states, actions, and rewards presented during real-world execution and retrain. \newline -- \textit{Sim-to-Real Transfer Techniques:} \newline Domain Adaptation: Use techniques like domain randomization and transfer learning to reduce the sim-to-real gap. 
\\
\hline
\multicolumn{3}{c}{} \\ % This adds an empty row with no lines
\end{tabular}

\end{table*}

\begin{table*}[h]
\caption{Goal 2 Responses for Case Study by C1}
\label{tab:goal2-res}
\footnotesize
\centering
\begin{tabular}{p{5.5cm}|p{5.5cm}|p{5.5cm}}
\rowcolor{BlueGray} \multicolumn{3}{c}{\textbf{Goal 2: Risk Management}} \\
\multicolumn{3}{c}{\textbf{\texttt{Subgoal 2.1 Risk-Aware Training}}} \\ \midrule

\textbf{\texttt{\uline{ASK 11:}} Do the training and evaluation metrics explicitly include measures across robustness, safety, and generalizability?} & \textbf{\texttt{\uline{ASK 12:}} Are safety constraints explicitly incorporated into the training process to effectively minimize risky behaviors?} & \textbf{\texttt{\uline{ASK 13:}} Does the reward function explicitly prioritize safety, incentivizing stable behavior and penalizing high-risk actions?} \\ 

\ding{51} \texttt{Yes} \ding{111} \texttt{No} \ding{111} \texttt{N/A} \ding{111} \texttt{?} & \ding{51} \texttt{Yes} \ding{111} \texttt{No} \ding{111} \texttt{N/A} \ding{111} \texttt{?} & \ding{51} \texttt{Yes} \ding{111} \texttt{No} \ding{111} \texttt{N/A} \ding{111} \texttt{?} \\ 

{\small \textbf{Explanation:}} \raggedright \newline -- \textit{Training:} \newline 1) States: Do not allow states that violate a minimum distance threshold. Penalize any actions where agents attempt to transition into these ‘not allowed’ states. \newline 2) Constrained Policy Optimization \newline -- \textit{Metrics:} \newline 1) Collision Rate \newline 2) Actions that would result in Minimum Separation Distance violations & {\small \textbf{Explanation:}} \newline -- \textit{Penalize Agent for the following:} \newline 1) Collisions \newline 2) Penalties for violating minimum separation distances, with the penalty magnitude increasing as the violation severity increases & {\small \textbf{Explanation:}} \newline See ASK 12 \\ \hline

\multicolumn{3}{c}{\textbf{\texttt{Subgoal 2.2 Proactive Risk Aversion}}} \\ \midrule

\multicolumn{3}{p{16.5cm}}{\textbf{\texttt{\uline{ASK 10:}} Have safety constraints been clearly defined and enforced to prevent the RL agent from entering high-risk states or taking unsafe actions at runtime?}} \\ 

\multicolumn{3}{p{16.5cm}}{\ding{51} \texttt{Yes} \ding{111} \texttt{No} \ding{111} \texttt{N/A} \ding{111} \texttt{?}}\\ 

\multicolumn{3}{p{16.5cm}}{{\small \textbf{Explanation:}} \raggedright \newline -- \textit{Minimum Separation Distances:} Define and enforce minimum separation constraints between agents and obstacles. \newline -- \textit{Speed and Acceleration Limits:} Set maximum allowable speeds and acceleration to prevent loss of control. \newline -- \textit{Operational Boundaries:} Define areas where agents should not operate, similar to a geofence.}\\ \hline

\end{tabular}

\begin{tablenotes}
    \small \textit{* To conserve space, only unique responses are included as two of the ASKs had similar explanations as those from Goal 1}
\end{tablenotes}

\end{table*}

\begin{table*}
\caption{Goal 2 Responses for Case Study by C1}
\label{tab:goal3-res}
\centering
\footnotesize{ % Experimenting with small font
\begin{tabular}{p{5.5cm}|p{5.5cm}|p{5.5cm}}
\rowcolor{BlueGray} \multicolumn{3}{c}
{\textbf{Goal 3: Human-Centric Alignment \& Control}} \\
\multicolumn{3}{c}{\textbf{\texttt{Subgoal 3.1 Human Intervention}}} \\ \midrule

\multicolumn{3}{p{16.5cm}}{\textbf{\texttt{\uline{ASK 18:}} Have human interventions been identified \& supported by affordances?}} \\ 

\multicolumn{3}{p{16.5cm}}{\ding{51} \texttt{Yes} \ding{111} \texttt{No} \ding{111} \texttt{N/A} \ding{111} \texttt{?}}\\ 

\multicolumn{3}{p{16.5cm}}{{\small \textbf{Explanation:}} \raggedright \newline -- \textit{Manual Override Controls:} \newline 1) Human operator can take control at any time. \newline 2) Human operator can opt out any agent out of the RL system and fall back to fail-safe or human control.} \\ \hline

\multicolumn{3}{c}{\textbf{\texttt{Subgoal 3.2 Human Oversight}}} \\ \midrule

\textbf{\texttt{\uline{ASK 15:}} If possible, is the human overseer actively involved in shaping the training process to enhance transparency \& promote alignment with specific safety \& operation goals?} & \textbf{\texttt{\uline{ASK 16:}} Are critical factors or states that significantly impact behavior and safety highlighted for the human overseer?} & \textbf{\texttt{\uline{ASK 17:}} Are rewards, actions, and states exposed to the human overseer during runtime to enhance the interpretability of the agent’s decisions?} \\ 

\ding{111} \texttt{YES} \ding{55} \texttt{No} \ding{111} \texttt{N/A} \ding{111} \texttt{?} & \ding{51} \texttt{Yes} \ding{111} \texttt{No} \ding{111} \texttt{N/A} \ding{111} \texttt{?} & \ding{51} \texttt{Yes} \ding{111} \texttt{No} \ding{111} \texttt{N/A} \ding{111} \texttt{?} \\ 

{\small \textbf{Explanation:}} \newline Other than the initial design of states, actions, and rewards, there is no additional human input that shapes the training process. & {\small \textbf{Explanation:}} \newline -- \textit{Display Proposed Paths:} Display proposed paths for each agent onto the GUI. \newline -- \textit{Minimum Separation Distances:} Display the minimum separation distance for each drone at each epoch onto the GUI. \newline -- \textit{Events/RL Errors:} Display events or RL errors onto the GUI, such as when an RL agent is stuck on a local minima and needs to transition to a fail-safe. & {\small \textbf{Explanation:}} \newline Yes, both during runtime via GUI and logged persistently. \\ \hline

\multicolumn{3}{c}{\textbf{\texttt{Subgoal 3.3 Post-Mortem Analysis}}} \\ \midrule

\multicolumn{3}{p{16.5cm}}{\textbf{\texttt{\uline{ASK 14:}} Are clear and detailed logs, metrics, and indicators available to trace decision-making and facilitate analysis of issues post-mortem?}} \\ 

\multicolumn{3}{p{16.5cm}}{\ding{51} \texttt{Yes} \ding{111} \texttt{No} \ding{111} \texttt{N/A} \ding{111} \texttt{?}}\\ 

\multicolumn{3}{p{16.5cm}}{{\small \textbf{Explanation:}} \raggedright \newline -- \textit{State, Action, Rewards Logging:} Record states, actions, rewards, and their corresponding state transitions for each agent, all timestamped. \newline -- \textit{Drone Telemetry Data:} Record drone telemetry data, including position, velocity, and orientation. \newline -- \textit{Event Categorization:} Categorize events as normal operations, constraint violations, or system alerts. \newline -- \textit{Performance and Safety Metrics:} Log metrics like path efficiency, time to destination, and minimum separation distance violations (or actions that would have led to such violations, as fail-safes will prevent any unsafe action). \newline -- \textit{Replay System:} Implement a replay system to view drone state transitions and their actions.} \\ \hline

\end{tabular}

\end{table*}

\clearpage
\newpage
% Define the custom color
\definecolor{teal}{HTML}{9AB8C2}
\definecolor{green1}{HTML}{9CBCA3}
\definecolor{rosepink}{HTML}{d398cb}
\begin{figure*}[h]
    \centering
    % Three Stacked Subfigures in Color Boxes
    \begin{subfigure}{0.85\textwidth}
        \begin{tcolorbox}[colback=teal!20!white, colframe=teal!80!black, width=\textwidth, boxrule=0.3mm, left=1mm, right=1mm, top=1mm, bottom=1mm]
            \includegraphics[width=\textwidth]{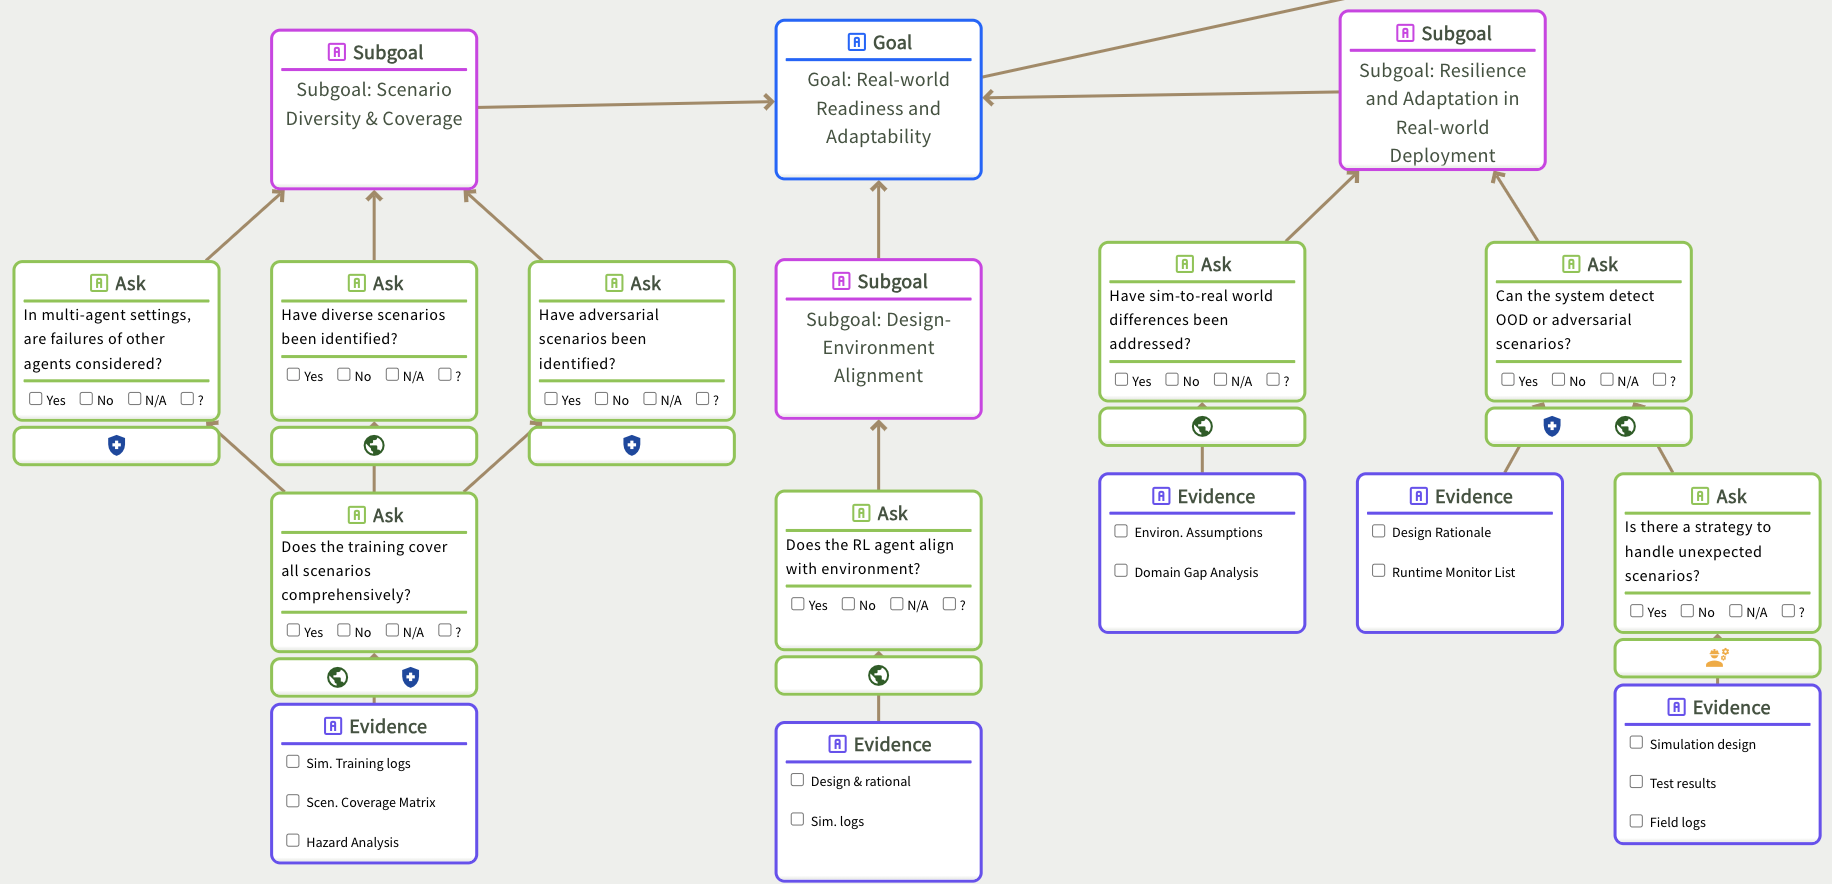} % Replace with your image path
        \end{tcolorbox}
        \caption{Goal 1}
    \end{subfigure}

    \begin{subfigure}{0.85\textwidth}
        \begin{tcolorbox}[colback=green1!10!white, colframe=green1!80!black, width=\textwidth, boxrule=0.5mm, left=1mm, right=1mm, top=1mm, bottom=1mm]
            \includegraphics[width=\textwidth]{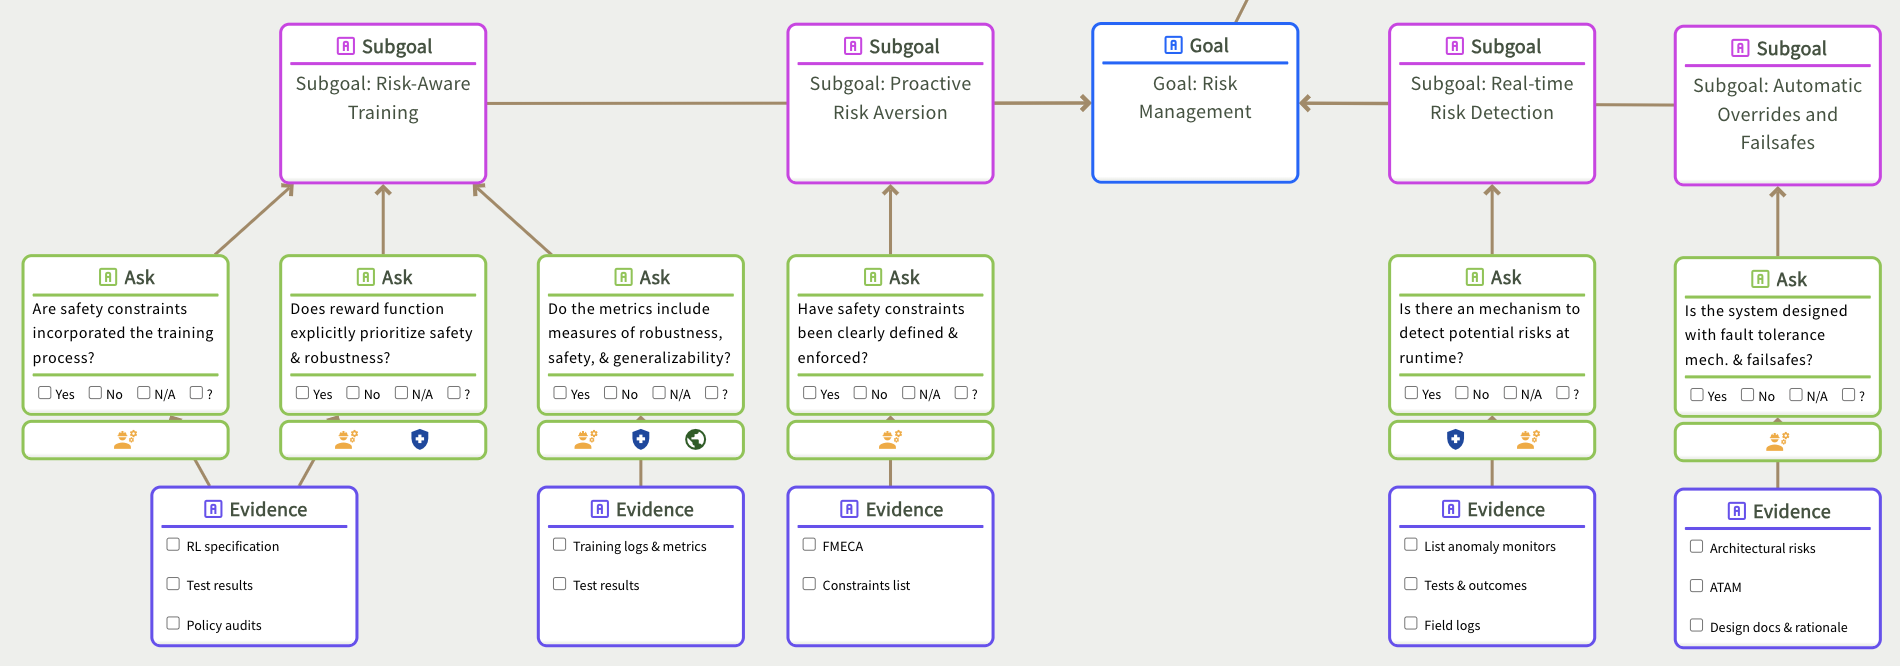} % Replace with your image path
        \end{tcolorbox}
        \caption{Goal 2}
    \end{subfigure}

    \begin{subfigure}{0.67\textwidth}
        \begin{tcolorbox}[colback=rosepink!10!white, colframe=rosepink!80!black, width=\textwidth, boxrule=0.5mm, left=1mm, right=1mm, top=1mm, bottom=1mm]
            \includegraphics[width=\textwidth]{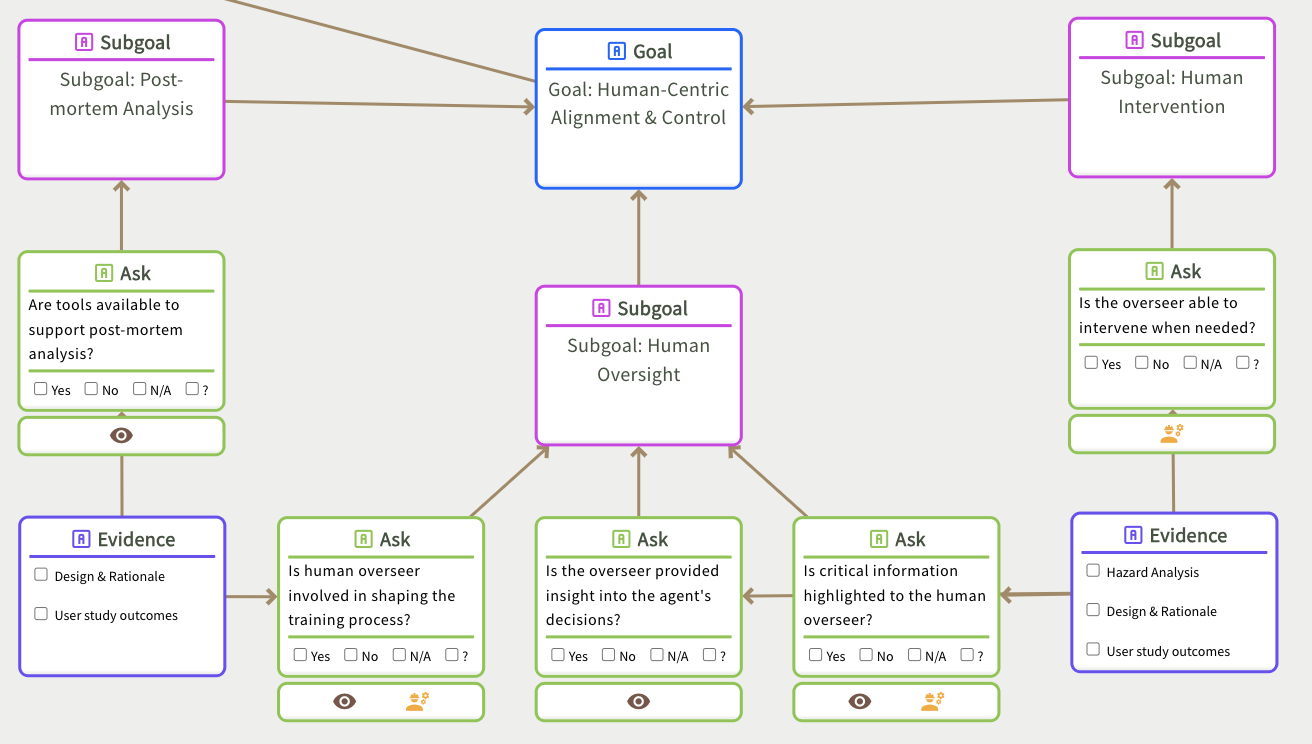} % Replace with your image path
        \end{tcolorbox}
        \caption{Goal 3}
    \end{subfigure}

    \caption{Subtrees of subgoals, \texttt{ASKS}, and evidence for the three top-level goals in the \framework framework.}
    \label{fig:goals-zoomed}
\end{figure*}
